# Supplementary material for: Bounded Invariant Checking for Stateflow Programs
Source: arXiv:2103.06248 source file (2021-11-19)
Supplement: Supplementary file 1 [file appendix-sos-rules.tex]

\section{Appendix: SOS rules}

In this section, we give the SOS rules \cite{hamon2004operationalsemanticsstateflow,hamon2007operationalsemanticsstateflow}, which we refer throughout the paper.

\begin{figure}[H]
    \centering
    \begin{minipage}{.5\textwidth}
    [t-FIRE]
    \begin{align*}
        \frac{e \vdash (c, D_1) \rightarrow{} true \quad\quad e \vdash (a, D_1) \hookrightarrow D_2}
        {e \vdash ((e_0, c, a_c, a_t, d), D_1) \rightarrow{} D_2, Fire(d, ta)}
    \end{align*}\newline
    
    [T-FIRE]
    \begin{align*}
        \frac{e \vdash (t, D_1) \rightarrow{} D_2, Fire(d, a)}
        {e, J \vdash (t.T, D_1) \rightarrow{} D_2, Fire(t.d, ta)}
    \end{align*}\newline
    
    [SD-FIRE]
    \begin{align*}
    \frac{\splitdfrac{e, J_0 \vdash (T_o, D_1) \rightarrow{} D_2, Fire(d, a) \quad e \vdash (a, D_2) \rightarrow{} D_3}
    {e \vdash (C, D_3) \Downarrow (C', D_4)
    {\quad e \vdash (A.x, D_4) \hookrightarrow{} D_5}}}
    %conclusion
    {e, J_0 \vdash ((A,C,T_i,T_o,J), D_1) \rightarrow{} ((A,C',T_i,T_o,J), D_5, Fire(d, \diamond))}
    \end{align*}\newline

[AND]
\begin{align*}
    \frac{\forall i \in [1,\dots n] \quad e,J \vdash (sd_i, D_i) \rightarrow{} (sd'_i,D_{i+1}, No)}
    %conclusion
    {\splitdfrac{e,J,tv \vdash (And\{s_0:sd_0 \cdots s_n:sd_n\}, D_1}{\rightarrow{} (And\{s_0:sd'_0 \cdots s_n:sd'_n\}, D_{n+1}, No)}}[*]
\end{align*}
\newline $[*]\:(tv_i = No) \lor (tv_i = End)$\newline

[OR-FIRE]
\begin{align*}
    \frac{e,J \vdash (sd, D_1)\rightarrow{} (sd', D_2, Fire(p', a))}
    %conclision
    {\splitdfrac{e, J, tv \vdash (Or(s,p,T,SD[s:sd]), D_1)}{\rightarrow{} (Or(\emptyset_s,p,T,SD[s:sd']), D_2, Fire(p',a))}}[*]
\end{align*}
[*] $[\mathit{(tv = No) \: \lor (tv = \: End), \quad \neg prefix(p',p)}]$
    \end{minipage}
    \caption{The subset of SOS rules used in our paper.}
  \label{fig:sos-rules-from-paper}
\end{figure}
